# Supplementary material for: Towards Reproducible Network Traffic Analysis
Source: arXiv:2203.12410 source file (2022-03-23)
Supplement: Supplementary file 1 [file appendix.tex]

\section{Appendix} \label{sec:appendix}

\subsection{\sys{} Live Traffic Encoding} \label{app:sys}

We now walkthrough an example of using \sys{} to encode metadata into
raw traffic captures \textit{in real time.}

\paragraph{Traffic Input.}
Traffic is captured from a supplied interface using the \texttt{libpcap}
library~\cite{libpcap}. We note here that running \sys{} in single-pcap 
mode and live mode is functionally the same, with the only difference
being reading from a saved traffic capture versus a live interface.

\paragraph{Metadata Inputs.}

When using \sys{} in live-capture mode, \sys{} supports defining traffic
samples via BPF filters, start and end timestamps, or any combination of
the two. Below is an example of a simple metadata file using BPF filters to capture
and encode metadata for ICMP and HTTPS traffic. 

\begin{lstlisting}[caption=An example metadata file when using pcapml in live-capture or single-pcap mode.]
\$ cat metadata.csv
bpf_filter,timestamp_start,timestamp_end,metadata #optional CSV header
ICMP,,,ICMP
port 22,,,SSH
\end{lstlisting}

\paragraph{\sys{} Attaching Metadata.}

Next, we run \sys{}, which generates a unique sampleID for each traffic sample
by hashing each metadata line in the metadata file. \sys{} then reads in 
traffic from the live interface and uses the filters (BPF or timing) to filter
traffic for each sample appropriately. Below is the command for running \sys{}
in live-capture mode using the example metadata file above.

\begin{lstlisting}[caption=Encoding a datset with metadata using pcapml.]
\$ pcapml -L metadata.csv -W live-dataset.pcapng
\end{lstlisting}

\paragraph{Output.}

\sys{} outputs a PCAPNG traffic capture file with metadata and sampleIDs
encoded for each filter supplied in the input metadata file. Below shows
the output of running the above command for a brief period using \texttt{tcpdump}.

\begin{lstlisting}[caption=pcapml-encoded files are portable to other tools.]
\$ tcpdump -r live-dataset.pcapng -n -c 10
20:10:59.278570 IP 128.112.224.83.22 > 10.8.59.231.58948: ...
20:10:59.282543 IP 10.8.59.231.58948 > 128.112.224.83.22: ...
16:27:53.949591 IP 10.8.59.231 > 128.112.224.83: ICMP echo request ...
16:27:53.949619 IP 128.112.224.83 > 10.8.59.231: ICMP echo reply ...
17:39:28.915687 IP 10.8.59.231 > 128.112.224.83: ICMP echo request ... 
17:39:28.915712 IP 128.112.224.83 > 10.8.59.231: ICMP echo reply ...
20:02:38.836711 IP 10.8.59.231.58948 > 128.112.224.83.22: ... 
20:02:38.837039 IP 128.112.224.83.22 > 10.8.59.231.58948: ...
\end{lstlisting}

The encoded metadata is easily viewable using \texttt{tshark}.

\begin{lstlisting}[caption=tools such as tshark can be used to directly inspect pcapml-encoded PCAPNGs.]
\$ tshark -r live-dataset.pcapng -T fields -e frame.comment
 14811793065302233675,SSH
 14811793065302233675,SSH
 8583516521062365758,ICMP
 8583516521062365758,ICMP
 8583516521062365758,ICMP
 8583516521062365758,ICMP
 14811793065302233675,SSH
 14811793065302233675,SSH
\end{lstlisting}

\paragraph{\sys{} Sorting Mode.}

By default, \sys{} outputs the traffic in timeseries order. In many cases,
users will desire the output to be first grouped by sampleID and \textit{then}
in timeseries order. The command below re-sorts the traffic in this manner.

\begin{lstlisting}
\$ pcapml -M live-dataset.pcapng -s -W sorted-live-dataset.pcapng
\end{lstlisting}

The output PCAPNG file is now sorted first by sampleID, and then by timestamp,
as shown below.

\begin{lstlisting}
\$ tcpdump -r sorted-live-dataset.pcapng
20:02:39.064070 IP 10.8.59.231.58948 > 128.112.224.83.22: ... 
20:02:39.059204 IP 128.112.224.83.22 > 10.8.59.231.58948: ...
20:02:39.058982 IP 10.8.59.231.58948 > 128.112.224.83.22: ...
20:02:38.844331 IP 10.8.59.231.58948 > 128.112.224.83.22: ...
20:02:38.837039 IP 128.112.224.83.22 > 10.8.59.231.58948: ...
20:02:38.836711 IP 10.8.59.231.58948 > 128.112.224.83.22: ...
20:10:59.282543 IP 10.8.59.231.58948 > 128.112.224.83.22: ...
20:10:59.278570 IP 128.112.224.83.22 > 10.8.59.231.58948: ...
17:39:28.915712 IP 128.112.224.83 > 10.8.59.231: ICMP echo reply
17:39:28.915687 IP 10.8.59.231 > 128.112.224.83: ICMP echo request
16:27:53.949619 IP 128.112.224.83 > 10.8.59.231: ICMP echo reply
16:27:53.949591 IP 10.8.59.231 > 128.112.224.83: ICMP echo request

\$ tshark -r sorted-live-dataset.pcapng -T fields -e frame.comment
14811793065302233675,SSH
14811793065302233675,SSH
14811793065302233675,SSH
14811793065302233675,SSH
14811793065302233675,SSH
14811793065302233675,SSH
14811793065302233675,SSH
14811793065302233675,SSH
8583516521062365758,ICMP
8583516521062365758,ICMP
8583516521062365758,ICMP
8583516521062365758,ICMP
\end{lstlisting}

\paragraph{Reverse Mode.} 

The \sys{} encoded dataset generated above can be split into multiple PCAP files,
one traffic file per sample with the single command shown below.

\begin{lstlisting}
\$ pcapml -M sorted-live-dataset.pcapng -O output_dir/
\end{lstlisting}
